# Supplementary material for: Probabilistic Visual Navigation with Bidirectional Image Prediction
Source: arXiv:2003.09224 source file (2022-02-18)
Supplement: Supplementary file 1 [file 5_supplemental_nc.tex]

%
%\section{Supplemental Material}
%
\subsection{Overriding in Trajectory Selection Module}
Our method can detect the obstacle and try to avoid it by considering the traversability score $S_{i, j}^{trav}$ based on GONet in the TS module.
However, the traversability score $S_{i, j}^{trav}$  occasionally fails for dynamic obstacles, e.g., pedestrians.
If a pedestrian suddenly appears in front of the robot, it is difficult for the robot to find the direction for the subgoals because there is insufficient space between the robot and the obstacle to take collision-free motion.
Moreover, adjacent obstacles occlude the appearance of the subgoal image from the current camera view.
The TS module in Fig. \ref{f:block_diagram} overrides the selected velocity to avoid the suddenly appeared obstacle as follows.
\begin{eqnarray}
\label{eq:sa_2}
    &&\hspace{-10mm}(v_t, \omega_t) = \nonumber \\ 
    &&\hspace{-5mm} \left\{
    \begin{array}{ll}
        (v_{i^\star, j^\star, 0}, \omega_{i^\star, j^\star, 0}) & \hspace{-2mm} : \hat{p}^{trav}_{t} \geq 0.5 \\
        (0.0, 0.5) & \hspace{-2mm} : \hat{p}^{trav}_{t} < 0.5 \hspace{1mm} \& \hspace{1mm} \theta_{i^\star, j^\star} \geq 0.0 \\
        (0.0, -0.5) & \hspace{-2mm} : \hat{p}^{trav}_{t} < 0.5 \hspace{1mm} \& \hspace{1mm} \theta_{i^\star, j^\star} < 0.0
    \end{array}
    \right. 
    %\nonumber \\
    %&&
\end{eqnarray}
where $\theta_{i^\star, j^\star} = \sum_{k=0}^{2L-1} \Delta_t \cdot \omega_{i^\star, j^\star, k}$, and traversable probability $\hat{p}^{trav}_{t}$ at the current position can be estimated by GONet\cite{hirose2018gonet}.
\begin{eqnarray}
\label{eq:sa_gonet}
\hat{p}^{trav}_{t} = f_{GONet}(I_t^f) 
\end{eqnarray}
The controller above makes the robot turn in place for at least three steps, corresponding to 90 degrees of rotation, when the area in front of the robot is untraversable.
The turning direction of the robot is decided by the sign of $\theta_{i^*, j^*}$, which is the yaw angle of the robot at the 2$L$-th future step on the robot coordinates.
Via this override, the robot tries to find the traversable area and capture the same appearance in the subgoal image.

Further, this controller limits the maximum linear velocity for the safety experiment at inference time.
$v_t$ is limited within $\pm$0.2 m/s and $\omega_t$ is set as $0.2 / r_t$ to keep the original turning radius $r_t = v_t / \omega_t$ when $|v_t| > 0.2$. 

\subsection{Illustration of trajectory likelihood}
Figure \ref{f:ex_eq} indicates the relationship between positions $\bar{x}_{i,j,k}$, $x_{i,j,k}$, and $x_{i,j,k}^{ref}$ and velocities $\bar{v}_{i, j, k-1}$, $u_{i, j, k-1}$, and $u_{i, j, k-1}^{ref}$ to illustrate the trajectory likelihood.
To learn the distribution of the teleoperator's velocity commands recorded in the dataset, our control policy generates the virtual mean robot pose $\bar{x}_{i,j,k}$ and its covariance matrix $P_{i,j,k}$ to fit with samples of the teleopeartor trajectory $x_{i,j,k}^{ref}$.
\subsection{Velocity Vector Selection}
Our method provides a distribution of velocity at each step.
At inference time, we generate several candidate velocities to select optimal velocities in the selection module.
However, the calculation cost to generate and evaluate a larger number of velocity vectors will be heavier and will impede the online calculation in the real robot.
Hence, we select only three velocity vectors $\nu_{i,j}$, with $j\in \{0\ldots M-1\}$ for each subgoal to perform our method online.
To obtain a wide variety of trajectory by three velocity vectors to avoid collision, we sample the following velocity at $k$ step according to $\{\mu_{i, j, k}\}_{j=0, 1, 2}$ and  $\{\Sigma_{i, j, k}\}_{j=0, 1, 2}$. % in (Eqn.~\ref{eq:polinet3_2}).
%In order to obtain as different trajectories as reachable with the 3 velocity vectors $\{\bm{u}_{i, j}\}_{j = 0, 1, 2}$, each velocity vector employs the velocity based on the following equation at each step.
%
\begin{eqnarray}
\label{eq:vv_select}
u_{i, 0, k} &=& \mu_{i, 0, k}, \nonumber\\
u_{i, 1, k} &=& \mu_{i, 1, k} + 2 \sqrt{\Sigma_{i, 1, k}} \left[ \begin{array}{c} 0 \\ 1 \end{array} \right], \\
u_{i, 2, k} &=& \mu_{i, 2, k} - 2 \sqrt{\Sigma_{i, 2, k}} \left[ \begin{array}{c} 0 \\ 1 \end{array} \right], \nonumber
\end{eqnarray}
where $\sqrt{\Sigma_{i, j, k}}$ is the square root of $\Sigma_{i, j, k}$, which is calculated by a solution such as a Cholesky decomposition.
Here $u_{i, 0, k}$, $u_{i, 1, k}$ and $u_{i, 2, k}$ are the mean, $+2$ sigma-points, and $-2$ sigma-points of the velocity distribution, respectively.
Note that only the sigma-points corresponding to the angular velocity are used, because the sigma-points corresponding to the linear velocity mostly cannot provide meaningful candidates for collision avoidance.
We consider that by taking a wide candidate in the angular velocity direction, the possibility of avoiding large obstacles would increase.
\begin{figure}[t]
  \begin{center}
  %\vspace*{-5mm}
      \includegraphics[width=0.9\hsize]{fig/ex_eq4.pdf}
  \end{center}
	\caption{\small {\bf Illustration of trajectory likelihood.} {Relationship between positions $\bar{x}_{i,j,k}$, $x_{i,j,k}$, and $x_{i,j,k}^{ref}$ and velocities $\bar{v}_{i, j, k-1}$, $u_{i, j, k-1}$, and $u_{i, j, k-1}^{ref}$.}}
  \label{f:ex_eq}
  %\vspace*{-3mm}
\end{figure}

As shown in Fig. \ref{f:overview_dist}, we repeatedly calculate (Eqn.~\ref{eq:vv_select}) for $2L$ steps to obtain three velocity vectors $\nu_{i,j}$, with $j\in \{0\ldots M-1\}$.
Despite the mean and distribution of velocity at the first step $k = 0$ being the same for all velocity vectors ($(\mu_{i, 0, 0}, \Sigma_{i, 0, 0}) = (\mu_{i, 1, 0}, \Sigma_{i, 1, 0}) = (\mu_{i, 2, 0}, \Sigma_{i, 2, 0})$), the three velocity vectors can cover a wide range of space to avoid large obstacles by repeatedly selecting the mean and $\pm$2 sigma-points for 2$L$ steps in (Eqn.~\ref{eq:vv_select}).
%the velocities at step $k > 0$ are selected from different velocity distributions depending on previous selected velocities.
%As the result, we can have wide variety of velocity vector for collision avoidance.
%This is because more various trajectory can be obtained by changing the angular velocity compared to the trajectory obtained by changing the linear velocity.

%Velocity vectors are generated by selecting the same sigma point repeatedly at each step ($k = 0, \cdots, 2N - 1$) as shown in (\ref{eq:vv_select}).

%The trajectories generated by selected 3 velocity vectors are shown in Fig. \ref{f:overview_dist}.
%
\begin{figure}[t]
  \begin{center}
  %vspace*{-5mm}
      \includegraphics[width=0.9\hsize]{fig/ex_dist2.pdf}
  \end{center}
	\caption{\small {\bf Velocity vector selection at inference time.} Double circles, red dots, and blue dots are position by mean velocity $u_{i, 0, k}$, $+2$ sigma-point velocity $u_{i, 1, k}$, and $-2$ sigma-point velocity $u_{i, 2, k}$, respectively. Grey, red, and blue lines indicate trajectories generated by velocity vectors $\nu_{i, 0}$, $\nu_{i, 1}$, and $\nu_{i, 2}$, respectively.}
  \label{f:overview_dist}
  \vspace*{-3mm}
\end{figure}
\begin{table*}[h]
  \caption{{\small Condition of cost value $J$ and visual localization approach in ablation study}}
  \begin{center}
  \resizebox{1.4\columnwidth}{!}{
  \label{tab:abcon}
  \begin{tabular}{l|cccc|cc|cc} \hline
    & \multicolumn{4}{c|}{(P)} & \multicolumn{2}{c}{(B)} &\multicolumn{2}{|c}{(S)} \\ \cline{2-9}
    & $J^{\textrm{\it tl}}$ & $J^{\textrm{\it smo}}$ & $J^{\textrm{\it imi}}$ &$J^{\textrm{\it trav}}$ & $J^{\textrm{\it bimg}}$ & $J^{\textrm{\it img}}$ & virt. vel. & pix. diff.  \\ \hline
    +P & \checkmark & \checkmark & & & & \checkmark & & \checkmark \\ \hline
    +B & & & \checkmark & \checkmark & \checkmark & & & \checkmark \\ \hline
    +S & & & \checkmark & \checkmark & & \checkmark & \checkmark & \\ \hline
    +P+B & \checkmark & \checkmark & & & \checkmark & & & \checkmark \\ \hline
    +P+S & \checkmark & \checkmark & & & & \checkmark & \checkmark & \\ \hline
    +B+S & & & \checkmark & \checkmark & \checkmark & & \checkmark & \\ \hline
    +P+B+S & \checkmark & \checkmark & & & \checkmark & & \checkmark & \\ \hline
  \end{tabular}
  }
  \end{center}
\end{table*}
\subsection{Alternative Method in Ablation Study}
In an ablation study, we evaluate all different sets of (P) probabilistic control, (B) bidirectional prediction, and (S) subgoal selection based on virtual velocities.
In the main paper, we omitted the detailed explanation of alternative methods where not all components are used.

\subsubsection{Without probabilistic control (P)}
The method without (P) has a deterministic control policy, which does not generate multiple velocities by setting $N = M = 1$.
Here $N$ is the number of subgoal images fed into the control policy, and $M$ is the number of generated virtual velocity vectors in the control policy. 
Hence, there is no TS module in the method without (P) because we have no choices from which to select the best one.
As a result, we remove the trajectory likelihood loss $J^{\textrm{\it tl}}$ from $J$ and add the following simple imitation loss $J^{imi}$.
\begin{eqnarray}
\label{eq:imiloss}
&&\hspace{-8mm}J^{\textrm{\it imi}}=\frac{1}{L}\sum_{k=0}^{L-1} (u^{ref}_{i, j, k} - u_{i, j, k})^2
\end{eqnarray}
The minimization of $J^{\textrm{\it imi}}$ has the effect of generating continuous virtual velocity, because the teleoperator's command is continuous.
Hence, we remove $J^{\textrm{\it smo}}$ when giving $J^{\textrm{\it imi}}$.
By minimization of cost value with $J^{\textrm{\it imi}}$, we train the model of control policy.
At inference time, we calculate the trained model to generate the deterministic virtual velocity with $N=M=1$.
%In addition, the model of control policy without (P) is simplified as follows:
%
%\begin{eqnarray}
%\label{eq:polinet3_1}
%\{u_{i,j,k}\}_{k=0 \cdots N}= f_{cp}^{woP}(I_t, I_{s+i}),
%\end{eqnarray}
%
%where $f_{cp}^{woP}()$ is a neural network by 7 convolutional layers with batch normalization and leaky relu function except last layer.
%Last layer does not have batch normalization and has hyperbolic tangent to limit the linear and angular velocity.

In contrast, the method without (P) cannot check the traversability, because there is no TS module.
To overcome this unfair condition, we give additional traversability loss $J^{\textrm{\it trav}}$ using GONet\cite{hirose2018gonet} when training the control policy like \cite{hirose2019dvmpc}.
\begin{eqnarray}
\label{eq:jgonet}
J^{\textrm{\it trav}} = \frac{1}{L} \sum_{k=0}^L(1 - \hat{p}^{'\textrm{\it trav}}_{t+k})^2
\end{eqnarray}
Here $\hat{p}^{'\textrm{\it trav}}_{t+k}$ is the kernelized traversable probability as $\hat{p}^{'\textrm{\it trav}} = \textrm{\it Clip}(\kappa^{\textrm{\it trav}}\cdot\hat{p}^{\textrm{\it trav}})$.
The kernelization helps the optimization to generate a virtual velocity that avoids areas of traversability smaller than $1/\kappa^{\textrm{\it trav}}$\cite{hirose2019dvmpc}.
\subsubsection{Without Bidirectional Prediction (B)}
To avoid using bidirectional prediction, we train the control policy with the following image loss $J^{\textrm{\it img}}$ instead of bi-directional image loss $J^{\textrm{\it bimg}}$ in $J$ for the method without (B).
\begin{eqnarray}
\label{eq:jpixel}
J^{\textrm{\it img}} = \frac{1}{L\cdot N_{\textrm{\it pix}}} \sum_{k=1}^L w_i(|I_{s+i} - \hat{I}_{t+k}|)
\end{eqnarray}
Here, $\{w_k\}_{k=1 \cdots L} = 1.0$ except $w_L = 5.0$ and $\{\hat{I}_{t+k}\}_{k=1 \cdots L}$ are predicted by VUNet-360 as shown in (Eqn.~\ref{eq:vunet2_f}).
$J^{\textrm{\it img}}$ calculates the pixel difference between the subgoal images $I_{s+i}$ and the predicted image $\{\hat{I}_{t+k}\}_{k=1 \cdots L}$.
By minimization of $J$ with $J^{\textrm{\it img}}$, the method without (B) can go to the position of subgoal $I_{s+i}$.
In addition, we choose $L=8$ for the method without (B), because the method of $L=8$ is better than that of $L=16$ from Table \ref{tab:ev} and Fig. \ref{f:ev_result}.
\subsubsection{Without Subgoal Selection Based on Virtual Velocity (S)}
The method without (S) evaluates the pixel difference between the current image view and the subgoal image to decide whether the robot is close to the subgoal or not.
The smaller pixel difference roughly means that the Euclidean distance between the robot position and subgoal position is shorter. 
The following equation is the condition to update the subgoal to the next one.
%According to the following equation, we basically update the subgoals by measuring the similarity between current image view and subgoal image.
%
\begin{eqnarray}
\label{eq:jpixel}
\frac{1}{N_{\textrm{\it pix}}} |I_{s+i} - I_{t}| < p_{th}
\end{eqnarray}
Here $p_{th}$ is the same threshold value as \cite{hirose2019dvmpc}.
The alternative method of (S) used in the ablation study is computationally as light as our method using virtual velocity.
\vspace{2mm}

Table \ref{tab:abcon} summarizes the cost value $J$ to train the control policy and selected method of (S) for all different sets of (P), (B), and (S) in the ablation study.
\subsection{Examples of simulation environment}
Figure \ref{f:env_sim} shows three examples of simulation environment\cite{xia2018gibson}.
Left photo depicts top view of the environment and visual trajectory.
Right photo depicts six subgoal image examples selected from all subgoals on the visual trajectory.
Map in left photo is taken by slicing the simulation environment at a certain height.
Hence, some furniture are not appeared on the map.
From Fig. \ref{f:env_sim}, We can understand that our method needs to pass through narrow doors and corridors to go to the goal position.
It means that environment even without obstacle occludes the appearance of the subgoal image view from the camera image view during navigation.
In that situation, bidirectional prediction can help to go through the narrow area.
The effectiveness of our method in the environment without presence of many obstacles is also shown in Fig.\ref{f:ev_result}.
Our method shows small advantage against strongest baseline at $l_{ob}$ = 1.0 and 1.5, where the obstacle is far from the subgoal image position, and achieve 0.992 goal arrival rate at $l_{ob}$ = 1.0 and 1.5.
\begin{figure}[t]
  \begin{center}
  \vspace*{-5mm}
  %\hspace*{-5mm}
    \begin{tabular}{c}
        \includegraphics[width=0.95\hsize]{fig/caseA.pdf} \\
        $\left[ \mbox{a} \right]$ case A : path length 8.6 m \\
        \\
        \includegraphics[width=0.95\hsize]{fig/caseB.pdf} \\
        $\left[ \mbox{b} \right]$ case B : path length 7.3 m \\
        \\
        \includegraphics[width=0.95\hsize]{fig/caseC.pdf} \\
        $\left[ \mbox{b} \right]$ case C : path length 11.9 m \\        
    \end{tabular}
  \end{center}
	\caption{\small {\bf Examples of simulation environment and rendered images.} Left photo depicts top view of the environment. Grey line is the visual trajectory, and grey dots on the grey line are the position of the subgoals. Right photos depict 6 subgoal image examples by 360 degree camera.}
  \label{f:env_sim}
  %\vspace*{-3mm}
\end{figure}
\subsection{Overview of different mobile robot}
Figure \ref{f:ev_b4d4} indicates the overview of the in-house prototype mobile robot, which was not used to collect the dataset.
This robot has a different mechanical structure, inertia, weight, sensor position, and so on compared to TurtleBot 2.
To validate the capability of our method, we test on this robot in the evaluation section. Our method works well on the new robot as well, because it arrives at the goal region with a success rate of 0.8.
\begin{figure}[t]
  \begin{center}
  %\vspace*{-5mm}
      \includegraphics[width=0.85\hsize]{fig/b4d4.pdf}
  \end{center}
      \vspace*{-4mm}
	\caption{\small {\bf Overview of the second prototype robot.} [a] shows the front view of the robot, [b] shows its back view. Unlike TurtleBot2, this robot has two front wheels and one rear omnidirectional wheel. We use the same laptop PC with the new robot and place the 360-degree camera in the front.}
  \label{f:ev_b4d4}
\end{figure}
